# Supplementary material for: Making Secure Software Insecure without Changing Its Code: The Possibilities and Impacts of Attacks on the DevOps Pipeline
Source: arXiv:2201.12879 source file (2022-01-30)
Supplement: Supplementary file 1 [file appendix1.tex]

\begin{table*}[tbh]
        \centering
          \caption{Threat Assessment Research}
\label{tab:threatModelComp}  
%\resizebox{\textwidth}{!}{%\vspace{.1in}
\begin{tabular}{|p{0.1\textwidth}|p{0.3\textwidth}|p{0.3\textwidth}|p{0.05\textwidth}|p{0.17\textwidth}| }

\hline 
\rowcolor{gray!18}
 \begin{center}
\textbf{{\small System}}
\end{center}
& \begin{center}
\textbf{{\small Potential Flaw}}
\end{center}
 & \begin{center}
\textbf{{\small Threat Description}}
\end{center}
 & \begin{center}
\textbf{{\small Risk Rating}}
\end{center}
 & \begin{center}
\textbf{{\small Mitigation Plan}}
\end{center}
 \\
\hline

Developer& Bad code commit& Dev pushes code with potential backdoor/malware& H& Place sanitation checks\\
\hline
& Code Injection& Injecting a malicious payload into code to trigger when it hits Git/Jenkins& H& Implement code sanitation checks\\
\hline
Git& Account Compromise& Potential privileged account compromise& L& Enable 2 factor auth\\
\hline
& Data in transit& Pushing/Pulling data from Git is transferred to source& M& Security gateway packets, ensure traffic is sent via TLS\\
\hline
& Vulnerable dependencies& Creating/Pulling docker container w vulnerable/malicious dependency& H& Vuln scan to verify docker containers\\
\hline
& Improper user of .gitignore& Upload undesired files giving potential sensitive info& M& Assure .gitignore has correct checks in place\\
\hline
Kubernetes& DDOS& Front end apps externally exposed& L& Proper security checks (ex. check in place to prevent multiple auth)\\
\hline
& Patching& K8s version depreciate& M& Maintain versions of K8s with latest security patches\\
\hline
& Ingress& Default ingress is not TLS& H& Set option for TLS\\
\hline
& Loadbalancer/Nodeport& Default to using specified port& H& Create route with TLS\\
\hline
& Secret Storage& Secrets stored in cleartext/unencrypted storage& H& Implement vault addon to secure secrets\\
\hline
& Kubeconfig file& Kubeconfig file contains details to manipulate the cluster& L& Implement RBAC, Follow Least Privileges\\
\hline
& Container exec& Accounts with various permissions might be able to escalate privileges& H& Implement RBAC, Follow Least Privileges\\
\hline
\multicolumn{3}{l}{} \\

% \hline
\end{tabular}%
%}
\end{table*}

\begin{table*}[tbh]
        \centering
          \caption{Threat Assessment Research}
\label{tab:threatModelComp2}  
%\resizebox{\textwidth}{!}{%\vspace{.1in}
\begin{tabular}{|p{0.1\textwidth}|p{0.3\textwidth}|p{0.3\textwidth}|p{0.05\textwidth}|p{0.17\textwidth}| }

\hline 
\rowcolor{gray!18}
 \begin{center}
\textbf{{\small System}}
\end{center}
& \begin{center}
\textbf{{\small Potential Flaw}}
\end{center}
 & \begin{center}
\textbf{{\small Threat Description}}
\end{center}
 & \begin{center}
\textbf{{\small Risk Rating}}
\end{center}
 & \begin{center}
\textbf{{\small Mitigation Plan}}
\end{center}
 \\
\hline
Jenkins& Control over CI/CD& Account can be used to alter build configs& L& Enable 2 factor auth\\
\hline
& Patching& Jenkins version depreciated& M& Maintain security patching\\
\hline
& Plugin Patching& Jenkins plugins become depreciated& H& Maintain security patching of plugins\\
\hline
Docker& Docker Pull& Potential infected container& M& Implement vuln scanning for containers\\
\hline
& Docker Build& Building container with vulnerable/malicious dependencies& H& Implement checks and detonation environment to test container\\
\hline
& Docker Run& Possible detonation of payload when container is run& H& Implement detonation zone to test containers\\
\hline
\multicolumn{3}{l}{} \\

% \hline
\end{tabular}%
%}
\end{table*}

\begin{table*}[tbh]
        \centering
          \caption{Threat Assessment Research}
\label{tab:threatModelComp3}  
%\resizebox{\textwidth}{!}{%\vspace{.1in}
\begin{tabular}{|p{0.1\textwidth}|p{0.3\textwidth}|p{0.3\textwidth}|p{0.05\textwidth}|p{0.17\textwidth}| }

\hline 
\rowcolor{gray!18}
 \begin{center}
\textbf{{\small System}}
\end{center}
& \begin{center}
\textbf{{\small Potential Flaw}}
\end{center}
 & \begin{center}
\textbf{{\small Threat Description}}
\end{center}
 & \begin{center}
\textbf{{\small Risk Rating}}
\end{center}
 & \begin{center}
\textbf{{\small Mitigation Plan}}
\end{center}
 \\
\hline
Strimzi& Network Policy& Default pods can access listeners& L& Configure proper network policy\\
\hline
& Internal plain listener& Allows for creation of unencrypted listener& L& Opt to create TLS listener\\
\hline
& Ingress& Ingress not TLS by default& H& Set to TLS on creation\\
\hline
& Loadbalancer/Nodeport& Listens on specified port by default& H& Create route with TLS instead\\
\hline
& Authentication for Listeners& Default listeners not using authentication& H& Options to setup authentication for listeners\\
\hline
& SuperUser compromise& SuperUsers have full access to cluster& H& Setting up proper RBAC\\
\hline
& JMX Port& JMX port not secure by default& L& JmxOptions allow for setting secure controls\\
\hline
& Pod Distribution& Default Strimzi allows for only 1 pod to be down& H& Setting PodDisruptionBudget allows for more tolerance\\
\hline
& SASL Plain& Allowed option to send creds over plaintext& H& Assure SASL encrypted method enabled\\
\hline
\multicolumn{3}{l}{} \\

% \hline
\end{tabular}%
%}
\end{table*}
